# Supplementary material for: FusionSF: Fuse Heterogeneous Modalities in a Vector Quantized Framework for Robust Solar Power Forecasting
Source: arXiv:2402.05823 source file (2024-02-08)
Supplement: Supplementary file 1 [file 3_related_works.tex]

\section{Related works}
Solar power forecasting is a thriving topic in the domain of energy forecasting~\cite{aReviewOfSolarForecasting}. Researches mainly focus on how to utilize advanced statistical and machine learning models to the specific application. There are ewo main branches of the work, one is to consider solar power curve as a time series and adopts time series forecasting methods, and the other is to find a map from metrological factors to the solar power and use regression methods~\cite{wu2022completed}.
\subsection{Deep networks for time series forecasting}

Solar power generation forecasting can be approached in two ways: pure time series forecasting or spatio-temporal forecasting, the latter incorporating geographical information. Deep neural networks, particularly Transformers, have garnered significant attention in the realm of time series forecasting~\cite{TransformerTS-Survey}. Several efficient and high-performance Transformers have been developed for this purpose, such as Informer~\cite{haoyietal-informer-2021}, Autoformer~\cite{Autoformer}, FEDformer~\cite{FedFormer}, FiLM~\cite{Film}, and PatchTST~\cite{patchTST}. Concurrently, fully connected models (like Dlinear~\cite{Dlinear} and LightTS~\cite{LightTS}) and Convolutional Neural Networks (CNNs) based models (like TimesNet~\cite{TIMESNET}) have also emerged as competitive alternatives in time series forecasting.

In the domain of spatio-temporal forecasting, it is a prevalent practice to employ a Unet~\cite{Unet} backbone and CNN structure to facilitate a hierarchical extraction of image features. To extract temporal information, 

one option is to employ convolution to build a Translator module, as demonstrated in the SimVP model~\cite{SimVP}. E3D-LSTM~\cite{3dlstm}  involves using 3D convolution which considers both spatial and temporal dependencies simultaneously. Alternatively, ConvLSTM~\cite{convlstm} utilize Recurrent Neural Networks (RNNs) to capture temporal dependencies and combines them with CNNs to capture spatial dependencies. 

Transformer-based models represent another family of methods that possess the potential to address both temporal and spatial dependencies. However, Transformers suffer from the quadratic complexity issue, which limits their scalability to large image inputs. A common approach is to divide the large input image into smaller patches, like in Earthformer~\cite{earthformer}. Leveraging the idea of patching, Pangu~\cite{PanguWeather} has developed a large-scale global weather forecasting model, which has yielded superior performance compared to conventional numeric weather prediction (NWP) methods. Despite the remarkable success in time series and spatio-temporal forecasting achieved by deep neural networks, handling solar power forecasting can still pose challenges, especially when there is a lack of diverse data sources to support the predictions.

\subsection{Multi-modality spatio-temporal}

Traditional methods typically focus on constructing a regression model that directly correlates the NWP data with solar power generation. However, the effectiveness of these methods heavily depends on the accuracy of weather reports. To address this limitation, \cite{MM-SkyImage-SolarIrradiance} incorporates sky images as an additional input for solar power prediction. By utilizing a Vision Transformer to analyze sky images and an Informer~\cite{haoyietal-informer-2021} model to handle solar power time series data, this approach strives to provide valuable vision insights for more accurate solar power predictions. However, it is worth noting that not all solar power stations are equipped with sky cameras capable of capturing sky images to a particular site. CrossViVit~\cite{crossvivit} introduces the satellite image as surrounding physical context, with a particular focus on cloud cover. CorssViVit employs a cross-attention mechanism to effectively combine the two modalities, and use ROtary positional encoding to handle the coordinates information of solar sites and satellite images.

\subsection{Zero shot learning for time series}
A recent work~\cite{LLM-zeroshot-ts} involves encoding time series as prompt and leveraging the power of large language models (LLMs) for zeroshot learning. Nonetheless, this approach falls short compared to certain specialized time series models. Despite the existence of robust zero-shot learners for natural language, achieving zeroshot learning for time series remains challenging. This difficulty primarily arises from the distribution disparities among time series originating from different domains. However, in the domain zero-shot learning is possible. N-BEATS~\cite{N-beats-zeroshot} act as a meta-learning adaptation and demonstrates remarkable zeroshot performance in the domain of finance (M3 \& M4 dataset). OneFitsAll extensively evaluates several SOTA TS models and proves that deep Transformer structure (GPT2) to be the best zeroshot learner. CrossViVit~\cite{crossvivit} proves the zeroshot ability for multi-modality forecasting.
